# Supplementary material for: Retrieve in Style: Unsupervised Facial Feature Transfer and Retrieval
Source: arXiv:2107.06256 source file (2021-08-24)
Supplement: Supplementary file 2 [file supp2_t.tex]

\begin{figure*}[thb]
    \centering
    \includegraphics[width=1\linewidth]{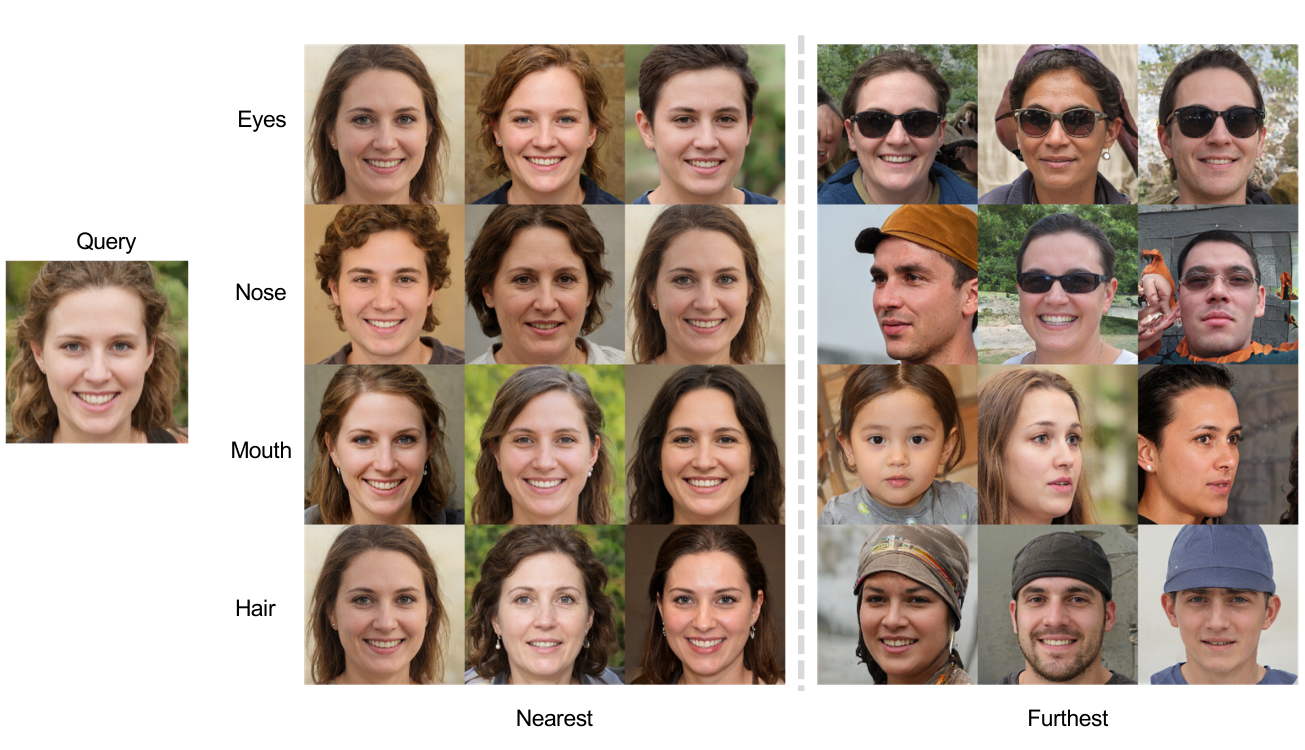}
    \caption{Results of retrieval on generated images.}
    \label{fig:supp2}
\end{figure*}
